# Supplementary material for: Variational Autoencoding of PDE Inverse Problems
Source: arXiv:2006.15641 source file (2020-06-28)
Supplement: Supplementary file 1 [file algorithm.tex]

\begin{algorithm}[H]
    \SetAlgoLined
    \DontPrintSemicolon
    \KwResult{Mini-patch estimate of $\mathbb{E}\left[\| \mathcal{R}(\bz)\|^2 \right]$} \;
    
    $\hat{r} \leftarrow 0$
    
    \For{$p \leftarrow 1$ \KwTo $P$}{
    
        \tcc{Perform local assembly}
        \For{$i \sim \mathrm{Unif}(\mathbb{N})$, $k \in \{i\}\cup \Nei{i}$}{
            \For{$l \in \mathbb{T}^{\text{active}}$}{
            $$
            (\mathbf{L}[\bz_m]^{(i)})_{kl} \leftarrow 
            \int_{\Omega} \mathcal{L}[\bz_m] \varphi_l \varphi_k dx
            $$}
            $(\bff^{(i)})_k \leftarrow \int_{\Omega} f \varphi_k$ dx\;
        }
        \tcc{Gather from forward surrogate}
        \For{$l \in \mathbb{T}^{\text{active}}$}{
            $(\boldsymbol{\mu}^{(i)} )_l \leftarrow 
            \mu(\bar{\bx}_l, \mathbf{z}_m)$
        }

        \tcc{Update MC estimate}
        $\hat{r} \leftarrow \hat{r} + P^{-1} r^{(i)}(\bz_m ; 
        \mathbf{L}^{(i)}, \bff^{(i)}, \boldsymbol{\mu}^{(i)})$
    }
\caption{Mini-patch Monte-Carlo estimate of $\mathcal{R}(\bz)$.}
\end{algorithm}
